# Supplementary material for: About evaluation metrics for contextual uplift modeling
Source: arXiv:2107.00537 source file (2021-08-02)
Supplement: Supplementary file 1 [file appendix_nu.tex]

\section{Variance reduction with $V_\nu$ }
\label{appendix:nu}

\subsection{Distributions}

We define the underlying distributions of $(X,T,Y)$:
\begin{itemize}
    \item i.i.d.~context features $X \sim \mathcal D_X$ in~$\X$
    \item treatment $T \sim \text{Ber}(\alpha)$ where $\alpha$ is the propensity to be treated (independent of $X=x$, (RCT assumption)
    \item outcome $Y \sim \mathcal D_Y(\cdot | X=x, T=t)$
\end{itemize}

We denote the resulting distribution over triples~$(X, T, Y)$ as $\mathcal D_\pi$.
The following proof is valid for mono context $X=x_0$, i.e. nothing is contextual, but generalizes easily in the contextual setting.
The conditional outcome r.v. $Y|T$ is Bernoulli distributed: $Y|T=0 \sim \text{Ber}(p_0)$ and $Y|T=1 \sim \text{Ber}(p_1)$. Think of $p_1-p_0>0$ as being the uplift.

\subsection{Estimators for $V_1$ and $V_2$ rules}

Let $Q_1$ be the estimator of the increment presented as $V_1$ rule, and $Q_2$ be the estimator of the increment presented as $V_2$ rule. With a balanced treatment/control distribution (i.e $\alpha = 0.5$), we can use:
\begin{itemize}
    \item $Q_1 = Y(2T-1)$
    \item $Q_2 = (Y-1)(2T-1)$
\end{itemize}
But as shown in Sections \ref{sec:toy_ex2} and \ref{section:unbalanced_dataset}, for any other values of $\alpha$, the uplift curve should not be directly built with +1 or -1 increments. Instead, we have to re-balance the two populations by applying factors on the +1/-1 increments. Those factors are based on $\alpha$ when $T=1$ and on $1 - \alpha$ when $T=0$. The re-scaled increments are presented in the Table \ref{table:Q1_Q2}. Note that compared to Table \ref{table:V1_V2_rules}, we apply here an extra constant $1/2$ factor so that when $\alpha = 0.5$, we get the classical +1/-1 increments back. This $1/2$ factor does not actually change the result of this appendix.

\begin{table}[!ht]
\begin{center}
\begin{tabular}{ | c | c || c | c | c |c |}
 \hline
 Y & T & $V_1$ rules & $Q_1(\alpha)$ & $V_2$ rules & $Q_2(\alpha)$ \\
 \hline
 0 & 0 & 0 & 0 & $+1$ & $+\frac{1}{2 (1 - \alpha)}$\\ 
 0 & 1 & 0 & 0 & $-1$ & $-\frac{1}{2 \alpha}$\\  
 1 & 0 & $-1$ & $-\frac{1}{2 (1 - \alpha)}$ & 0 & 0 \\   
 1 & 1 & $+1$ & $+\frac{1}{2 \alpha}$ & 0 & 0 \\
 \hline
\end{tabular}
 \caption{$V_1$ and $V_2$ sets of rules, with $Q_1$ and $Q_2$ increments}
\label{table:Q1_Q2}
\end{center}
\end{table}

% \begin{table}[!ht]
% \begin{center}

% \begin{tabular}{ | c| c || c | c | c |} 
% \hline
% $Y$ & $T$ & $V_1$ rules & $V_2$ rules & weight \\ 
% \hline
% 0 & 0 & 0 & $+1$ & $1 / (2(1 - \alpha))$\\ 
% 0 & 1 & 0 & $-1$ & $1 / (2(1 - \alpha))$ \\
% 1 & 0 & $-1$ & 0 & $1 / (2 \alpha)$ \\
% 1 & 1 & $+1$ & 0 & $1 / (2 \alpha)$  \\
% \hline
% \end{tabular}
%  \caption{$V_1$ and $V_2$ sets of rules}
% \label{table:V1_V2_rules_var}
% \end{center}
% \end{table}

For the computation of the optimal $\nu$ that minimizes the variance of the barycentric estimator $Q[\nu]$, we need to compute first $\E[Q_1]$, $\E[Q_2]$, $\E[Q_1^2]$, and $\E[Q_2^2]$.

\begin{align*}
    \E[Q_1]=&\frac{1}{2 \alpha}P(Q_1=1/(2\alpha))-\frac{1}{2-2\alpha}P(Q_1=-1/(2-2\alpha))) \\
    =&\frac{1}{2 \alpha} \left(\cancel{P(Q_1=1/(2\alpha)|T=0)}P(T=0)+P(Q_1=1/(2\alpha)|T=1)P(T=1)\right)\\
    &-\frac{1}{2-2\alpha}\left(P(Q_1=-1/(2-2\alpha)|T=0)P(T=0)+\cancel{P(Q_1=-1/(2 -2\alpha)|T=1)}P(T=1)\right) \\
    =&\frac{1}{2 \alpha}\left(P(Y=1|T=1)P(T=1)\right)-\frac{1}{2 -2\alpha}\left(P(Y=1|T=0)P(T=0)\right) \\
    =& \frac{p_1 \alpha}{2\alpha} - \frac{p_0 (1 - \alpha)}{2-2\alpha} = \frac{p_1 - p_0}{2}
\end{align*}

\begin{align*}
    \E[Q_2]=&\frac{1}{2-2\alpha}P(Q_2=1/(2-2\alpha))-\frac{1}{2 \alpha}P(Q_2=-1/(2\alpha)) \\
    =&\frac{1}{2-2\alpha}\left({P(Q_2=1/(2-2\alpha)|T=0)}P(T=0)+\cancel{P(Q_2=1/(2-2\alpha)|T=1)}P(T=1)\right)\\
    &-\frac{1}{2 \alpha}\left(\cancel{P(Q_2=-1/(2\alpha)|T=0)}P(T=0)+{P(Q_2=-1/(2\alpha)|T=1)}P(T=1)\right) \\
    =&\frac{1}{2-2\alpha}\left(P(Y=0|T=0)P(T=0)\right)-\frac{1}{2 \alpha}\left(P(Y=0|T=1)P(T=1)\right) \\
    =&\frac{(1 - p_0)(1-\alpha)}{2-2\alpha}-\frac{(1 - p_1)\alpha}{2 \alpha} = \frac{p_1 - p_0}{2} = \E[Q_1]
\end{align*}

Thus: $$\E[Q_1] - \E[Q_2] = 0$$.

\begin{align*}
    \E[Q_1^2]=&\frac{1}{(2 \alpha)^2}P(Q_1=1/(2\alpha)^2)+\frac{1}{(2-2\alpha)^2}P(Q_1=1/(2-\alpha)^2) \\
    =&\frac{1}{(2 \alpha)^2} \left(\cancel{P(Q_1=1/(2 \alpha)^2|T=0)}P(T=0)+P(Q_1=1/(2 \alpha)^2|T=1)P(T=1)\right)\\
    &\frac{1}{(2-2\alpha)^2}\left(P(Q_1=1/(2-2\alpha)^2|T=0)P(T=0)+\cancel{P(Q_1=1/(2-2\alpha)^2)|T=1)}P(T=1)\right) \\
    =&\frac{1}{(2 \alpha)^2}\left(P(Y=1|T=1)P(T=1)\right)+\frac{1}{(2 -2\alpha)^2}\left(P(Y=1|T=0)P(T=0)\right) \\
    =& \frac{p_1 \alpha}{(2 \alpha)^2} + \frac{p_0 (1 - \alpha)}{(2 -2\alpha)^2} = \frac{p_1}{4\alpha} + \frac{p_0}{4 - 4\alpha}
\end{align*}

\begin{align*}
    \E[Q_2^2]=&\frac{1}{(2-2\alpha)^2}P(Q_2=1/(2-2\alpha)^2)+\frac{1}{(2 \alpha)^2}P(Q_2=1/(2 \alpha)^2) \\
    =&\frac{1}{(2-2\alpha)^2}\left({P(Q_2=1/(2-2\alpha)^2|T=0)}P(T=0)+\cancel{P(Q_2=1/(2-2\alpha)^2|T=1)}P(T=1)\right)\\
    &+\frac{1}{2 \alpha}\left(\cancel{P(Q_2=1/(2 \alpha)^2|T=0)}P(T=0)+{P(Q_2=1/(2 \alpha)^2|T=1)}P(T=1)\right) \\
    =&\frac{1}{(2-2\alpha)^2}\left(P(Y=0|T=0)P(T=0)\right) + \frac{1}{(2 \alpha)^2}\left(P(Y=0|T=1)P(T=1)\right) \\
    =&\frac{(1 - p_0)(1-\alpha)}{(2-2\alpha)^2}+\frac{(1 - p_1)\alpha}{(2 \alpha)^2} = \frac{1 - p_0}{4 - 4\alpha} + \frac{1 - p_1}{4\alpha}
\end{align*}

Thus: $$\E[Q_1^2] + \E[Q_2^2] = \frac{1}{4\alpha} + \frac{1}{4 - 4\alpha} = \frac{1}{4\alpha(1 - \alpha)}$$

\subsection{Barycentric estimator and optimal $\nu$}

$V_{\nu}$ is a barycentric combination of $V_1$ and $V_2$: $V_{\nu}=(1-\nu)V_1+\nu V_2$ with $\nu \in [0, 1]$.

Let $Q_{\nu}$ be its estimator: $Q_{\nu} = (1-\nu)Q_1+\nu Q_2$ with $\nu \in [0, 1]$.\\

Its variance is:
\begin{align*}
    Var(Q_{\nu})=& Var((1-\nu)Q_1+\nu Q_2) \\
    =&(1-\nu)^2 Var(Q_1)+\nu^2 Var(Q_2)+2(1-\nu)\nu Cov(Q_1,Q_2)
\end{align*}

Note that $Cov(Q_1,Q_2)=\cancel{\E[Q_1 Q_2]}-\E[Q_1]\E[Q_2]$.\\

Differentiating $\nu \mapsto Var(Q_{\nu})$ w.r.t. $\nu$ gives:
\begin{align*}
\frac{d(Var(Q_{\nu}))}{d(\nu)} &= -2(1-\nu)Var(Q_1)+2\nu Var(Q_2)+2(1-2\nu)Cov(Q_1,Q_2) \\
&= 2 \nu (Var(Q_1) + Var(Q_2) - 2 Cov(Q_1,Q_2)) -2 Var(Q_1) + 2 Cov(Q_1,Q_2)
\end{align*}
That is a linear function with a positive slope:
\begin{align*}
Var(Q_1) + Var(Q_2) - 2 Cov(Q_1,Q_2) &= \E[Q_1^2] - \E[Q_1]^2 + \E[Q_2^2] - \E[Q_2]^2 + 2 \E[Q_1]\E[Q_2] \\
&= \E[Q_1^2] + \E[Q_2^2] - (\E[Q_1] - \E[Q_2])^2 \\
&= \E[Q_1^2] + \E[Q_2^2] \\
&= \frac{1}{4\alpha(1 - \alpha)} > 0 \quad \forall \alpha \in (0, 1)
\end{align*}

Thus, solving $\frac{d(Var(Q_{\nu}))}{d(\nu)} = 0$ gives the $\nu$ value that minimizes $Var(Q_{\nu})$:

\begin{align*}
\nu=&\frac{Var(Q_1)-Cov(Q_1,Q_2)}{Var(Q_1)+Var(Q_2)-2 Cov(Q_1,Q_2)} \\
    =& \frac{\E[Q_1^2] - \E[Q_1]^2 + \E[Q_1] \E[Q_2]}{\E[Q_1^2] - \E[Q_1]^2 + \E[Q_2^2] - \E[Q_2]^2 + 2 \E[Q_1]\E[Q_2]} \\
    =& \frac{\E[Q_1^2] - \E[Q_1] (\E[Q_1] - \E[Q_2])}{\E[Q_1^2] + \E[Q_2^2] - (\E[Q_1] - \E[Q_2])^2} \\
    =& \frac{\E[Q_1^2]}{\E[Q_1^2] + \E[Q_2^2]} \\
    =& \left(\frac{p_1}{4\alpha} + \frac{p_0}{4 - 4\alpha}\right) 4\alpha (1 - \alpha) \\
    =& p_1(1-\alpha) + p_0 \alpha
\end{align*}

Or equivalently: $$\nu + P(Y=1) = p_0 + p_1$$

In particular, when $\alpha = 0.5$, we have $$\nu = \frac{p_0 + p_1}{2} = P(Y=1)$$
